# Supplementary material for: PrivacyGo: Privacy-Preserving Ad Measurement with Multidimensional Intersection
Source: arXiv:2506.20981 source file (2025-06-26)
Supplement: Supplementary file 1 [file 9_appendix.tex]

\section{Appendix}
\label{sec:appendix_dp_proof}
\subsection{Proof of Lemma~\ref{lemma:set_cdn_pmf}}
\label{app:pmf}
\begin{proof}
According to Algorithm~\ref{alg:DP-SI-SingleID}, it is established that both $D_A$ and $D_B$ are independent of both $A$ and $B$. Consequently, it becomes evident that
$|A_\mathsf{up}\cap B_\mathsf{up}|
=|A\cap B|+\mathsf z$,
where 
$
\mathsf z \triangleq |D_A\cap D_B|.
$

To calculate $\Pr(\mathsf{z} = z)$, we need to determine the number of outcomes where the intersection size of $D_A \cap D_B$ is $z$ and then divide by the total number of possible outcomes.
There are $\C_{2\tau}^\tau$ possible outcomes for both $D_A$ and $D_B$ since they constitute the first half of the random permutation result of $D$. Therefore, the total number of outcomes is $\C_{2\tau}^\tau \cdot \C_{2\tau}^\tau$.

The number of outcomes for $D_B$ alone is $\C_{2\tau}^\tau$. For any $|D_A \cap D_B| = z$, it implies that there are $z$ elements in $D_B$ belonging to $D_A$, with $\C_{\tau}^z$ possible outcomes. Simultaneously, the remaining $\tau - z$ elements in $D_B$ must be randomly selected from $D \setminus D_A$, offering $\C_{\tau}^{\tau - z}$ possibilities. Consequently, we can compute the PMF of $\mathsf{z} = |D_A \cap D_B|$ as follows:
$
\label{eq:PMF}
    \Pr(\mathsf z= z) =  \frac{\C_{2\tau}^\tau\C_{\tau}^z \cdot \C_\tau^{\tau-z}}{\C_{2\tau}^\tau\cdot\C_{2\tau}^\tau}= \frac{(\C_{\tau}^z)^2}{\C_{2\tau}^\tau}.
$
\end{proof}

\subsection{Proof of Property~\ref{prop:symmetric}}
\label{app:one-delta}
\begin{proof}
Denote {$\{0,...,\tau\}$} as the support of $\mathsf z$, the support of $\mathcal{M}(A)$ becomes: $\{|A\cap B|,...,|A\cap B|+\tau\}$.
Given the asymmetrically distributed property, we have $\Pr(\mathsf z = \tau-o) = \Pr(\mathsf z = o)$, $\forall{o\in[0,\tau]}$. Given the sensitivity of the operation of  $|A\cap B|$ is $1$, 
% Let $1$ be the sensitivity of the query (operating function) of $A$, i.e. $|A\cap B|$.
The worst-case neighboring dataset $\mathcal{M}(A^\prime)$ has the support of $\{|A\cap B|+1,..., |A\cap B|+\tau+1\}$, and the mapping relationships of the two neighboring datasets become
$ 
    \Pr(\mathcal{M}(A)=o) = \Pr(\mathcal{M}(A^\prime) = o+1).
$ 
Define ${O}$ as the support of the output of the mechanism, ${O}^+$ as the subset of ${O}$ corresponds to the criterion:
$ 
    O^+ = \{o: \Pr(\mathcal M(A)=o)-e^{\varepsilon} \Pr(\mathcal M(A^\prime)=o)\ge 0 \}.
$ 
Then, according to the definition of DP, the failure probability $\delta$ can be expressed as:
\begin{equation*}\label{eq:delta_expression}
\begin{aligned}
    \delta=&\sum_{o \in O} \max \left(\Pr(\mathcal M(A)=o)-e^{\varepsilon} \Pr(\mathcal M(A^\prime)=o), 0\right)\\
    =&\sum_{o\in{O}^+}\left(\Pr(\mathcal M(A)=o)-e^{\varepsilon} \Pr(\mathcal M(A^\prime)=o\right)\\
    =&\sum_{o\in{O}^+}\left(1-e^{\varepsilon}\frac{\Pr(\mathcal M(A^\prime)=o)}{\Pr(\mathcal M(A)=o)}\right)\Pr(\mathcal M(A)=o),
    \end{aligned}
\end{equation*}
% Given the definition of privacy loss distribution $\Pr(\bm \gamma=\gamma)$:
% \begin{equation*}
    % \Pr\left(\bm \gamma = \ln\left(\frac{\Pr(\mathcal{M}(A)=o)}{\Pr(\mathcal{M}(A')=o)}\right)\right)=\Pr(\mathcal{M}(A)=o)
% \end{equation*}
This shows how \eqref{eq:dp_profile} is derived.
% which can be further expressed as:
%     \begin{equation*}
% \begin{aligned}
%     \delta=& \sum_{\gamma:\gamma>\epsilon}(1-e^{\epsilon-\gamma})P_{\bm \gamma}(\gamma)\\
%     \triangleq &\Pr(\gamma=\infty) + \sum_{\gamma:\epsilon<\gamma<\infty}(1-e^{\epsilon-\gamma})P_{\bm \gamma}(\gamma),
% \end{aligned}
% \end{equation*}
% where the first part $\delta(\infty)$ captures the failures due to the uneven support of $\mathcal{M}(A)$ and $\mathcal{M}(A^\prime)$, where once happen, causes infinity leakage. The latter part $\delta(\bm \gamma>\epsilon)$ measures the integral of probability that the leakage is limited, but cannot be bounded by $\epsilon$.
For the first term in \eqref{eq:dp_profile}
\begin{equation}
\begin{aligned}
\delta_{AA'}(\infty)=&\sum_{\substack{\{o|\Pr(\mathcal{M}(A)=o)>0,\\ \Pr(\mathcal{M}(A^\prime)=o)=0\}}}\Pr(\mathcal{M}(A)=o)\\
=&\sum_{o=|A\cap B|}^{|A\cap B|}\Pr(\mathcal{M}(A)=o) \\
=&\Pr(\mathcal{M}(A)=|A\cap B|)
\end{aligned}
\end{equation}
For the other direction,
% For the first term in \eqref{eq:generaldelta}
\begin{equation}
\begin{aligned}
\delta_{A'A}(\infty)=&\sum_{\substack{\{o|\Pr(\mathcal{M}(A^\prime)=o)>0,\\ \Pr(\mathcal{M}(A)=o)=0\}}}\Pr(\mathcal{M}(A^\prime)=o)\\
% =&\sum_{o=\tau+1}^{\tau+1}\Pr(\mathcal{M}(A^\prime)=o)\\
=&\sum_{o=|A\cap B|+\tau}^{|A\cap B|+\tau}\Pr(\mathcal{M}(A)=o)\\
=&\Pr(\mathcal{M}(A)=|A\cap B| + \tau)\\
=&\Pr(\mathcal{M}(A)=|A\cap B|)\\
\end{aligned}
\end{equation}
which means $\delta_{AA'}(\infty) = \delta_{A'A}(\infty)$.

For the second part of \eqref{eq:dp_profile}, first, let $\bm \gamma_{AA'}(o)$ and $\bm \gamma_{A'A}(o)$ be:
\begin{equation*}
\begin{aligned}
&\bm \gamma_{AA'}(o) = \ln\left(\frac{\Pr(\mathcal{M}(A)=o)}{\Pr(\mathcal{M}(A^\prime)=o)}\right),\\
&\bm \gamma_{A'A}(o) = \ln\left(\frac{\Pr(\mathcal{M}(A^\prime)=o)}{\Pr(\mathcal{M}(A)=o)}\right)
\end{aligned}
\end{equation*}
Then, $\bm \gamma_{AA'}(o)=-\bm \gamma_{A'A}(o)$, and by the symmetric property, $\bm \gamma_{AA'}(o) = \bm \gamma_{A'A}(\tau+1-o)$. Then,
the second part $\delta(\bm \gamma>\epsilon)$ for each term can be expressed as:

\begin{equation*}
    \delta(\bm \gamma_{AA'}>\epsilon)=\sum_{o = 1}^{\bm \gamma_{AA'}^{-1}(\epsilon)}(1-e^{\epsilon-\bm \gamma_{AA'}(o)})\Pr(\mathcal{M}(A) = o)
\end{equation*}
and 
\begin{equation*}
\begin{aligned}
&\delta(\bm \gamma_{A'A}>\epsilon)\\
=&\sum_{o = \bm \gamma_{A'A}^{-1}(\epsilon)}^{\tau}(1-e^{\epsilon-\bm \gamma_{A'A}(o)})\Pr(\mathcal{M}(A^{\prime}) = o)\\
% =&\sum_{o = \bm \gamma_{A'A}^{-1}(\epsilon)}^{\tau}(1-e^{\epsilon-\bm \gamma_{A'A}(o)})\Pr(\mathcal{M}(A) = o-1)\\
% =&\sum_{o = \bm \gamma_{A'A}^{-1}(\epsilon)-1}^{\tau-1}(1-e^{\epsilon-\bm \gamma_{A'A}(o+1)})\Pr(\mathcal{M}(A) = o)\\
% =&\sum_{o = \tau-\bm \gamma_{AA'}^{-1}(\epsilon)}^{\tau-1}(1-e^{\epsilon-\bm \gamma_{AA'}(\tau-o)})\Pr(\mathcal{M}(A) = o)\\
=&\sum_{o = 1}^{\bm \gamma_{AA'}^{-1}(\epsilon)}(1-e^{\epsilon-\bm \gamma_{AA'}(o)})\Pr(\mathcal{M}(A) = o).
\end{aligned}
\end{equation*}
Therefore, $\delta(\bm \gamma_{AA'}>\epsilon)=\delta(\bm \gamma_{A'A}>\epsilon)$. 
\end{proof}
% \subsection{Proof of Property~\ref{prop: k-fold}}
% \todo[inline]{YJ: Pending inputs?}

\subsection{Proof of Property~\ref{prop: window}}
\label{app:window_len}
\begin{proof}
$W$ is lower bounded by the maximum leakage after $k$-fold convolution. From \eqref{eq:PLD1}, the maximum leakage of the mechanism can be expressed as
\begin{equation}
2\ln\left(\max_{z\in[0,\tau-1]} \frac{z+1}{\tau-z}\right)=2\ln(\tau)    
\end{equation}
The length of the PLD is:
\begin{equation}
2\ln\left(\max_{z\in[0,\tau-1]} \frac{z+1}{\tau-z}\right)-2\ln\left(\min_{z\in[0,\tau-1]} \frac{z+1}{\tau-z}\right)=4\ln{\tau}
\end{equation}
Then, the maximum leakage after $k$-fold composition becomes:
\begin{equation}
2\ln(\tau)+4(k-1)\ln(\tau)=(4k-2)\ln(\tau)
\end{equation}
% This completes the proof.
\end{proof}

\subsection{Security Proof for DPCA-PSI}\label{sec:appendix_proof}
This section contains the full version of the security proof of $\Pi_{\mathsf{DP-PSI}}$. 

We recall the definitions of computational differential privacy (CDP) and the view of protocol execution. 
%%%%%%%%%  Let's go with the ``Real/Ideal'' style of definition  %%%%%%%%%%%%%%%

\begin{definition}[The view of a protocol execution~\cite{cu/Goldreich2004}]\label{def:view}
Let $f: \{0,1\}^\ast \times \{0,1\}^\ast \rightarrow \{0,1\}^\ast \times \{0,1\}^\ast$ be a functionality, and $f_{P_A}(A,B)$ (resp., $f_{P_B}(A,B)$) denote the first (resp., second) element of $f(A,B)$. 
Let $\Pi$ be a two-party protocol for computing the function $f$.
The $\view$ of the first (resp., second) party during execution of $\Pi$ on $(A,B)$, denoted $\view^{\Pi}_{P_A}(A,B)$ (resp.,$\view^{\Pi}_{P_B}(A,B))$), is $(A, r, m_1, \ldots, m_t)$ (resp., $(B, r, m_1, \ldots, m_t)$), where $r$ represents the output of the first (resp., second) party's internal coin tosses, and $m_i$ represents the $i$-th message it has received. 
\end{definition}

\begin{definition}[$(\epsilon_\kappa, \delta)$-$\SIM$-$\cdp$ Privacy~\cite{crypto/MironovPRV09,eurosp/KacsmarKLNSSBSO20}]
\label{def:sim-cdp}
An interactive protocol ensemble $\{\langle f_\kappa(\cdot),g_\kappa(\cdot)\rangle\}_{\kappa \in \mathbb{N}}$, ensures for $\{f_\kappa\}_{\kappa \in \mathbb{N}}$ $(\epsilon_{\kappa}, \delta)$-$\SIM$-$\cdp$, if for every ensemble $\{g^*_\kappa\}_{\kappa \in \mathbb{N}}$ of efficiently computable randomized interactive functions, there exists an ensemble $\{F_\kappa\}_{\kappa \in \mathbb{N}}$ of $(\epsilon_\kappa, \delta)$-differentially-private mechanisms $F_\kappa(\cdot)$ such that for every $x \in \mathcal{D}$, the probability ensembles $\{VIEW_{\kappa, g^*_\kappa}(x)\}_{\kappa \in \mathbb{N}}$ and $\{F_\kappa(x)\}_{\kappa \in \mathbb{N}}$ are computationally indistinguishable.


% We say that a two-party protocol $\Pi_{f} : \mathcal{X}^m \times \mathcal{X}^n \rightarrow \mathcal{Z}$ ensures $(\epsilon, \delta)$-$\SIM$-$\cdp$ if there exists an $(\epsilon, \delta)$-DP (per Definition~\ref{def:eddp}) mechanism $\mathcal{\hat{F}}(\cdot, \cdot)$ such that for every input $(x, y) \in \mathcal{X}^m \times \mathcal{X}^n$, the probability ensembles $VIEW{}$

% the protocol $\Pi_{f}$ is a secure two-party computation protocol for the randomized functionality $\mathcal{\hat{F}}(\cdot, \cdot)$ as per the ``ideal/real''-style definition of secure two party computation~\cite{cu/Goldreich2004}. 
\end{definition}

Besides, the security of our protocols relies on the classic Decisional Diffie-Hellman (DDH) assumption:
\begin{definition}[DDH Assumption]\label{def:ddh}
Let $\GG$ be a group (parameterized by security parameter $\lambda$) and $g$ be a generator. We say that the~\emph{Decisional Diffie-Hellman (DDH)} assumption holds in group $\GG$ if for every PPT adversary $\mathcal{A}$:
$$
|\Pr[\mathcal{A}(g, g^a, g^b, g^{ab}) = 1] - \Pr[\mathcal{A}(g, g^a, g^b, g^c) = 1]| \leq \negl[\lambda],
$$
where the probability is taken over $a \leftarrow \ZZ_q$, $b \leftarrow \ZZ_q$, $c \leftarrow \ZZ_q$ and the random coins of $\mathcal{A}$. 
\end{definition}

We now prove the security in the semi-honest model, where we assume both parties follow the protocol steps honestly, but may try to extract as much information about the other party's private inputs as possible.
Due to the page limit, we refer readers to Appendix~\ref{sec:appendix_proof} for the full proof. In this section, we briefly summarize the corresponding theorem and our proof outline below.


\begin{theorem}[Security of $\Pi_{\mathsf{DPCA-PSI}}$]
\label{thm:dppsi}
The two-party protocol $\Pi_{\mathsf{DPCA-PSI}}$ ensures $(\epsilon, \delta)$-$\SIM$-$\cdp$ for both party $A$ and party $B$. 
\end{theorem}

Following the definition of SIM-CDP in Definition~\ref{def:sim-cdp}, the proof consists of two parts.
The first part of the proof shows that $\Pi_{\mathsf{DPCA-PSI}}$ is a secure two-party computation protocol that implements DPCA-PSI functionalities. The correctness of the protocol is straightforward as shown by the protocol description. To prove the privacy, we construct the protocol view (Figure~\ref{fig:view_a_1}) and the corresponding simulator $S$ (Figure~\ref{fig:sim_A_new}), then we illustrate that the distributions produced by them are computationally indistinguishable through a series of hybrid arguments. In general, we show that if the adversary can differentiate the outputs from the simulator and the view, the adversary can leverage it to break the DDH assumption. Besides, as $\Pi_{\mathsf{DPCA-PSI}}$ is a symmetric protocol in the sense that the operations of two parties are the same except the input, we only need to prove SIM-CDP for one of the parties, and the other party's proof is trivial by exchanging the roles of two parties in the proof.

The second part of the proof shows that $\Pi_{\mathsf{DPCA-PSI}}$ (and consequently, the simulator $S$) is an $(\epsilon, \delta)$-differentially private mechanism. As $\Pi_{\mathsf{DPCA-PSI}}$ correctly implements DPCA-PSI functionalities, this proof is reduced to the differential privacy proof of DPCA-PSI (Theorem~\ref{two_way_dp}). Consequently, as the simulator $S$ can only obtain the outputs of DPCA-PSI, which are $(\epsilon, \delta)$-differentially private, $S$ naturally achieves $(\epsilon, \delta)$ differential privacy as well.

\begin{proof}

As DPCI-PSI protocol is symmetric in the sense that both party A and party B run the same operations (but with different inputs), it is sufficient to provide security proof for party A, and the proof for party B is trivial by replacing party A with party B in the proof. 

First, we describe the protocol view $VIEW^{A}$ in \Cref{fig:view_a_1} to summarize the data that party A can access during the protocol execution. Then in~\Cref{fig:sim_A_new} we describe the simulator $\SIM_A$ (consistent with the definition of $F_\kappa(\cdot)$ in Definition~\ref{def:sim-cdp}), which simulates the protocol view without party B's input. We claim that the distribution generated by $\SIM_A$ in the ideal world is indistinguishable from the output distribution of party $A$ shown in $VIEW^{A}$. 

The outputs of $VIEW^{A}$ consist of three parts: (1) Party A's inputs, (2) Party A's randomness, and (3) Messages that party A receives from Party B. As (1) and (2) are available to both $VIEW^{A}$ and $\SIM_A$. We only need to prove that the distribution of the messages party A receives from party B in the actual protocol execution view $VIEW^{A}$ is computationally indistinguishable from the messages generated by $\SIM_A$. These messages include $H^1_{B2A}$, $(h_{\mathbf{a}_1})^{\alpha_1\beta_1}_{\pi_{B_1}}$, and $(h^\ell_{a2b,\ell})^{\alpha_1\beta_\ell}_{\pi_{B_\ell}}$, $(h^\ell_{b2a,\ell})^{\alpha_\ell\beta_\ell}_{\pi_{A_\ell}}$ for $\ell \in {2, 3, \ldots, L}$.  Our proof uses the standard hybrid argument, where the neighboring pair of hybrid distributions is (computationally) indistinguishable. The proof is inspired by~\cite{ion2020deploying}, which uses a similar approach to prove the security of PSI-SUM.



\begin{figure*}[tp] \footnotesize
    \centering

\fbox{

    \begin{minipage}{\textwidth} 
    
    \smallskip
    \textbf{Procedure $VIEW^{A}_{\Pi_{\mathsf{DPCA-PSI}}}(\mathsf{PII_A}, \mathsf{PII_B}, m, n, L, 
 \hat{c})$} 
    
    \smallskip
    \textbf{Inputs:}
    \begin{itemize}
        \item 
        Party $A$'s input: $\mathsf{PII_A} = [\mathbf{a}_1, \ldots, \mathbf{a}_L]$, where $\mathbf{a}_\ell = (\mathbf{a}_\ell[1], \ldots, \mathbf{a}_\ell[m])^T$ and $\mathbf{a}_\ell[i] \in \{0,1\}^\ast$ for $\ell \in [L], i \in [m]$;  
        
        \item  
         Party $B$'s input: $\mathsf{PII_B} = [\mathbf{b}_1, \ldots, \mathbf{b}_L]$, where $\mathbf{b}_\ell = \left(\mathbf{b}_\ell[1], \ldots, \mathbf{b}_\ell[n] \right)^T$ and $\mathbf{b}_\ell[i] \in \{0,1\}^\ast$ for $\ell \in [L], i \in [n]$. 

         \item $\hat{c} = [\hat{c}_1, \ldots, \hat{c}_L]$ is the output of $\Pi_{\mathsf{DPCA-PSI}}$.
    \end{itemize}
        \smallskip  \hrule \smallskip
    \textbf{Protocol:}
    \begin{itemize}
        \item \textbf{Step 0: Setup}
        \begin{itemize}
            \item $\alpha = (\alpha_1, \ldots ,\alpha_L)$ from $\ZZ_p^L$.
            \item $\beta = (\beta_1, \ldots ,\beta_L)$ from $\ZZ_p^L$.
        \end{itemize}
        \item \textbf{Step 1: Appending dummy items for differentially private set intersection size:}
        \begin{itemize}
            \item This steps requires no communication between Party A and Party B, thus it is a local computation and Party A simply follows the protocol honestly to generate the dummy.
        \end{itemize}

        \item \textbf{Step 2.1: Column-wise shuffling. For each column $\ell \in [L]$:}
            \begin{itemize}
                \item $\pi_A \xleftarrow[]{\$} \mathbb{P}_{m'}$, where $\mathbb{P}_{m'}$ represents all permutations with size $m'$
                \item $\pi_B \xleftarrow[]{\$} \mathbb{P}_{n'}$, where $\mathbb{P}_{n'}$ represents all permutations with size $n'$
                \item $\mathbf{a}_\ell = \pi_A(\mathbf{a}_\ell)$
                \item $\mathbf{b}_\ell = \pi_B(\mathbf{b}_\ell)$
            \end{itemize}
        \item \textbf{Step 2.2: Hashing all the elements.}  
            \begin{itemize}
            \item for $\ell \in [L], i \in [m']$, $\mathbf{a}_\ell[i] = H(\mathbf{a}_\ell[i])$
    
            \item for $\ell \in [L], i \in [n']$, $\mathbf{b}_\ell[i] = H(\mathbf{b}_\ell[i])$
            \item $H_A = [h_{\mathbf{a}_1}, \ldots, h_{\mathbf{a}_L}]$ such that $h_{\mathbf{a}_i} = [\mathbf{a}_i[0], \ldots, \mathbf{a}_i[m']]$ for $i \in L$
            \item $H_B = [h_{\mathbf{b}_1}, \ldots, h_{\mathbf{b}_L}]$ such that $h_{\mathbf{b}_i} = [\mathbf{b}_i[0], \ldots, \mathbf{b}_i[n']]$ for $i \in L$
            \end{itemize}
    
        \item \textbf{Step 3: finding matching records column-by-column in a "waterfall" process via Diffie-Hellman style key exchange}

            \begin{itemize}
                \item  Matching the 1st column: 
                \begin{itemize}
                    \item Get $H^1_{B2A} = [(h_{\mathbf{b}_1})^{\beta_1}, \ldots, (h_{\mathbf{b}_L})^{\beta_1}]$ from Party B, raise each value by the power of $\alpha_i$.
                    
                    \item $\pi_{A_1} \xleftarrow[]{\$} \mathbb{P}_{n'}$
                    \item $h^{1, \alpha_1, \pi_{A_1}}_{B2A} = \pi_{A_1}((h_{\mathbf{b}_1})^{\beta_1\alpha_1})$
                    \item $\pi_{B_1} \xleftarrow[]{\$} \mathbb{P}_{m'}$
                    \item $h^{1, \beta_1, \pi_{B_1}}_{A2B} = \pi_{B_1}((h_{\mathbf{a}_1})^{\alpha_1\beta_1})$
                    \item compute the intersection of $(h_{\mathbf{b}_1})^{\alpha_1\beta_1}$ and $h^{1, \beta_1, \pi_{B_1}}_{A2B}$, ~\ie, $h_{\cap, 1} = (h_{\mathbf{b}_1})^{\alpha_1\beta_1} \cap (h_{\mathbf{a}_1})^{\alpha_1\beta_1}_{\pi_{B_1}}$. 
                        Let $\idx_1 = \phi$ be an empty set and $\tilde{c}_1 = |h_{\cap, 1}|$. \\
                        For all $(h_{\mathbf{b}_1}[i])^{\alpha_1\beta_1} \in h_{\cap, 1}$, party $A$ marks the $i$-th row of $H^1_{B2 A}$ as ``deleted'' and adds $i$ to $\idx_1$. Party $A$ further marks the first column of $H^1_{B2A}$ as ``deleted''. Let $H^2_{B2A} = [(h^2_{b2a,2})^{\beta_1}, \ldots, (h^2_{b2a, L})^{\beta_1}] \in \GG^{(n'-\tilde{c}_1)\times(L-1)} $ denote the remaining matrix (after removing the column and rows marked as ``deleted'').
                \end{itemize}
                \item Step 3.2:  Matching from the second column to the $L$-th column. For $\ell = 2$ to $L$:
                    \begin{itemize}
                        \item Let $H^{\ell}_{B2A}= [(h^\ell_{b2a,\ell})^{\beta_1}, \ldots, (h^\ell_{b2a, L})^{\beta_1}]$ denote the remaining matrix at party $A$ after columns and rows removal in the previous matching;
                        \item $\pi_{A_\ell}, \pi_{B_\ell} \xleftarrow[]{\$} \mathbb{P}$
                        \item $h^{\ell, \alpha_\ell, \pi_{A_\ell}}_{B2A} = \pi_{A_\ell}(h_{(\mathbf{b}_\ell})^{\beta_1\alpha_\ell})$, $h^{\ell, \beta_\ell, \pi_{B_\ell}}_{A2B} = \pi_{B_\ell}((h_{\mathbf{a}_\ell})^{\alpha_1\beta_\ell})$
                        %\item  \xleftarrow[]{\$} \mathbb{P}$
                        %\item $h^{\ell, \beta_\ell, \pi_{B_\ell}}_{A2B} = \pi_{B_\ell}((h_{\mathbf{a}_\ell})^{\alpha_1\beta_\ell})$
                        \item $H_{\ell, A2B} = (h^{\ell, \beta_\ell, \pi_{B_\ell}}_{A2B})^{\alpha_\ell\alpha_1^{-1}} = \pi_{B_\ell}((h_{\mathbf{a}_\ell})^{\alpha_\ell\beta_\ell})$, $H_{\ell, B2A} = (h^{\ell, \alpha_\ell, \pi_{A_\ell}}_{B2A})^{\beta_\ell\beta_1^{-1}} = \pi_{A_\ell}((h_{\mathbf{b}_\ell})^{\alpha_\ell\beta_\ell})$
                %        \item $H_{\ell, B2A} = (h^{\ell, \alpha_\ell, \pi_{A_\ell}}_{B2A})^{\beta_\ell\beta_1^{-1}} = \pi_{A_\ell}((h_{\mathbf{b}_\ell})^{\alpha_\ell\beta_\ell})$
                        \item Party A reverts the permutation $\pi_{A_\ell}$ to get back $(h_{\mathbf{b}_\ell})^{\alpha_\ell\beta_\ell}$ and computes the intersection $h_{\cap, \ell} = (h_{\mathbf{b}_\ell})^{\alpha_\ell\beta_\ell} \cap H_{\ell, A2B}$.
                        \item For all elements in $(h_{\mathbf{b}_\ell})^{\alpha_\ell\beta_\ell}$ that lie in the intersection $h_{\cap, \ell}$, party $A$ recovers the corresponding index back in $H^1_{B2A}$ and adds the index to $\idx_\ell$. Party $A$ further marks those rows as ``deleted'' and removes the $\ell$-th column in $H^1_{B2A}$. Let $H^{\ell+1}_{B2A}$ denote the remaining matrix after removal;
                    \end{itemize}
            \end{itemize}
 
        \item \textbf{Step 4: output}
        \begin{itemize}
            \item Party $A$ outputs $L$ integers $(\tilde{c}_1, \ldots, \tilde{c}_L)$, where $\tilde{c}_\ell = |h_{\cap, \ell}|$ for all $\ell \in [L]$ computed from above.
        \end{itemize}

        \item \textbf{The output of $VIEW^{A}_{\Pi_{\mathsf{DPCA-PSI}}}$ includes the following three parts:}
        \begin{itemize}
            \item Party A's input: $\mathsf{PII_A}$
            \item Party A's randomness: $\alpha = (\alpha_1, \ldots ,\alpha_L)$
            \item Messages that party A receives: $H^1_{B2A}$, $(h_{\mathbf{a}_1})^{\alpha_1\beta_1}_{\pi_{B_1}}$, $(h_{a2b,\ell})^{\alpha_1\beta_\ell}_{\pi_{B_\ell}}$, $(h_{b2a,\ell})^{\alpha_\ell\beta_\ell}_{\pi_{A_\ell}}$ for $\ell \in {2, 3, \ldots, L}$.
        \end{itemize}
    \end{itemize}
    \end{minipage}
}

    \caption{Party A's view for computing $\Pi_{{\mathsf{DPCA-PSI}}}$}
    \label{fig:view_a_1}
\end{figure*}


% \begin{figure*}[tp] \footnotesize
%     \centering

% \fbox{

%     \begin{minipage}{\textwidth} 
    
%     \smallskip
%     \textbf{Part 2: Procedure $VIEW^{A}_{\Pi_{\mathsf{DPCA-PSI}}}(\mathsf{PII_A}, \mathsf{PII_B}, m, n, L, 
%  \hat{c})$} 

    
%     \begin{itemize}
 
%         \item \textbf{Step 3.2:  Matching from the second column to the $L$-th column. For $\ell = 2$ to $L$:}
%         \begin{itemize}
%             \item Let $H^{\ell}_{B2A}= [(h^\ell_{b2a,\ell})^{\beta_1}, \ldots, (h^\ell_{b2a, L})^{\beta_1}]$ denote the remaining matrix at party $A$ after columns and rows removal in the previous matching;
%             \item $\pi_{A_\ell}, \pi_{B_\ell} \xleftarrow[]{\$} \mathbb{P}$
%             \item $h^{\ell, \alpha_\ell, \pi_{A_\ell}}_{B2A} = \pi_{A_\ell}(h_{(\mathbf{b}_\ell})^{\beta_1\alpha_\ell})$, $h^{\ell, \beta_\ell, \pi_{B_\ell}}_{A2B} = \pi_{B_\ell}((h_{\mathbf{a}_\ell})^{\alpha_1\beta_\ell})$
%             %\item  \xleftarrow[]{\$} \mathbb{P}$
%             %\item $h^{\ell, \beta_\ell, \pi_{B_\ell}}_{A2B} = \pi_{B_\ell}((h_{\mathbf{a}_\ell})^{\alpha_1\beta_\ell})$
%             \item $H_{\ell, A2B} = (h^{\ell, \beta_\ell, \pi_{B_\ell}}_{A2B})^{\alpha_\ell\alpha_1^{-1}} = \pi_{B_\ell}((h_{\mathbf{a}_\ell})^{\alpha_\ell\beta_\ell})$, $H_{\ell, B2A} = (h^{\ell, \alpha_\ell, \pi_{A_\ell}}_{B2A})^{\beta_\ell\beta_1^{-1}} = \pi_{A_\ell}((h_{\mathbf{b}_\ell})^{\alpha_\ell\beta_\ell})$
%     %        \item $H_{\ell, B2A} = (h^{\ell, \alpha_\ell, \pi_{A_\ell}}_{B2A})^{\beta_\ell\beta_1^{-1}} = \pi_{A_\ell}((h_{\mathbf{b}_\ell})^{\alpha_\ell\beta_\ell})$
%             \item Party A reverts the permutation $\pi_{A_\ell}$ to get back $(h_{\mathbf{b}_\ell})^{\alpha_\ell\beta_\ell}$ and computes the intersection $h_{\cap, \ell} = (h_{\mathbf{b}_\ell})^{\alpha_\ell\beta_\ell} \cap H_{\ell, A2B}$.
%             \item For all elements in $(h_{\mathbf{b}_\ell})^{\alpha_\ell\beta_\ell}$ that lie in the intersection $h_{\cap, \ell}$, party $A$ recovers the corresponding index back in $H^1_{B2A}$ and adds the index to $\idx_\ell$. Party $A$ further marks those rows as ``deleted'' and removes the $\ell$-th column in $H^1_{B2A}$. Let $H^{\ell+1}_{B2A}$ denote the remaining matrix after removal;
%         \end{itemize}
%         \item \textbf{Step 4: output}
%         \begin{itemize}
%             \item Party $A$ outputs $L$ integers $(\tilde{c}_1, \ldots, \tilde{c}_L)$, where $\tilde{c}_\ell = |h_{\cap, \ell}|$ for all $\ell \in [L]$ computed from above.
%         \end{itemize}

%         \item \textbf{The output of $VIEW^{A}_{\Pi_{\mathsf{DPCA-PSI}}}$ includes the following three parts:}
%         \begin{itemize}
%             \item Party A's input: $\mathsf{PII_A}$
%             \item Party A's randomness: $\alpha = (\alpha_1, \ldots ,\alpha_L)$
%             \item Messages that party A receives: $H^1_{B2A}$, $(h_{\mathbf{a}_1})^{\alpha_1\beta_1}_{\pi_{B_1}}$, $(h_{a2b,\ell})^{\alpha_1\beta_\ell}_{\pi_{B_\ell}}$, $(h_{b2a,\ell})^{\alpha_\ell\beta_\ell}_{\pi_{A_\ell}}$ for $\ell \in {2, 3, \ldots, L}$.
%         \end{itemize}
%     \end{itemize}
%     \end{minipage}
% }

%     \caption{Party A's view for computing $\Pi_{{\mathsf{DPCA-PSI}}}$ (Part 2)}
%     \label{fig:view_a_2}
% \end{figure*}


\begin{figure*}[tp] \footnotesize
\centering
\fbox{
    \begin{minipage}{0.9\textwidth}
    \textbf{Inputs:} $\mathsf{PII_A}=[\mathbf{a}_1, \ldots, \mathbf{a}_L]$, the noise number of matching record per column $(\hat{c}_1, \ldots, \hat{c}_L)$. 

    \begin{itemize}
        \item \textbf{Simulate Setup:}
            \begin{itemize}
                \item $\alpha = (\alpha_1, \ldots ,\alpha_L)$ from $\ZZ_p^L$.
                
                % \item To simulate the generation of $\beta$, the simulator $\SIM_A$ generates $L$ random elements from $\ZZ_p^L$: $\bar{\beta} = (\bar{\beta}_1, \ldots ,\bar{\beta}_L)$ where $\bar{\beta}_i \xleftarrow[]{\$} \ZZ_p^L$ for $i$ from $1$ to $L$. (We use bar symbol $\bar{x}$ to imply that the value $\bar{x}$ is generated by the simulator to simulate the value $x$ in actual execution).
            \end{itemize}            
        
        \item \textbf{Simulate Step 1:}
            \begin{itemize}
                \item In the protocol, party $B$ does not send any message to party $A$ in these two steps. $\SIM_A$ does not need to simulate party $B$'s action here and only need to perform the same steps as party $A$ honestly according to the protocol.  Hence, we skip the full details.
            \end{itemize}
            
        \item \textbf{Simulate Step 2:}
        This step aims at generating a fake input set of party B.
        \begin{itemize}
            \item $\SIM_A$ generates $\bar{H}_{B} \in \GG^{n' \times L} = {g_{ij}}$, where each $g_ij$ is randomly selected from $\GG$. 
            
            \item $\SIM_A$ generates $\bar{H}^\ast_{B}$ such that the following two constrains are satisfied: (1) the $j$-th column of $\bar{H}^\ast_{B}$ has $\hat{c}_j$ common elements with the $j$-th column of $\bar{H}_{B}$; (2) each row of $\bar{H}_{B}$ and $\bar{H}^\ast_{B}$ has at most one common element. The generation process is done as follows:
                    
                        \begin{enumerate}
                            \item For $j \in [L]$:
                            \item ~~~For $i \in [n']$:
                            \item ~~~~~~Let $\max = \sum^j_{k=1} \hat{c}_k$, $\min = \max - \hat{c}_j+1$;
                            \item ~~~~~~if $i \in [\min,\max]$, $\bar{H}^\ast_{B}[i,j] = g_{ij}$;
                            \item ~~~~~~else sample $\bar{H}^\ast_{B}[i,j]$ uniformly at random, \ie, $\bar{H}^\ast_{B}[i,j] \leftarrow \GG$. If the generated random value already exists in the column $j$, re-sample it until there is no collision.
                            \item Randomly shuffle all the rows of $\bar{H}^\ast_{B}$.
                        \end{enumerate}
        \end{itemize}

        
        \item \textbf{Simulate Step 3:}
            \begin{itemize}
                \item 1.Simulating the steps of matching the 1st column: 
                
                \begin{enumerate}
         
                    \item $\SIM_A$ sets fake message $\overline{H^1_{B2A}}$ = $\bar{H}^\ast_{B}$ and use it as party B's message in step 3.(i).
                    \item $\SIM_A$ follows the protocol description to perform Step 3.(ii).

                    \item $\SIM_A$ raises all elements in the first column of $\bar{H}_{B}$ to the power of $\alpha_1$, performs a random permutation $\bar{\pi}_B: [n'] \rightarrow [n']$ to it, then uses the result as party B's message $(h_{\mathbf{a}_1})^{\alpha_1\beta_1}_{\pi_{B_1}}$ in Step 3.(iii) of the real protocol execution. 
                                        
                    % \item $\SIM_A$ raises all elements in the first column of $\bar{H}_{B}$ to the power of $\alpha_1$, applies a random permutation and uses the result $\bar{H}_B[1]^{\alpha_1}_\bar{\pi}_B$ as party $B$ 's message $(h_{\mathbf{a}_1})^{\alpha_1\bar{\beta}_1}_{\bar{\pi}_{B_1}}$ in Step 3.(iii). 
                    
                    \item $\SIM_A$ follows the protocol description to perform Step 3.(iv).
                \end{enumerate}

                \item 2.Simulating the steps of matching the rest of the columns:

                \begin{enumerate}
                    \item $\SIM_A$ follows the protocol description to perform Step 3.(1) and (2) honestly. 
                       \item Let $\bar{H}^\ell_{B2A}$, which has $n'-\sum^{\ell-1}_{i=1} \hat{c}_i$ rows, denote the matrix that simulates $H^\ell_{B2A}$ in the real protocol. Note that $\SIM_A$ knows exactly which entries $\bar{H}^\ell_{B2A}[i',j']$ were set to be equal to $g_{i'j', A}$ and which were chosen uniformly at random. $\SIM_A$ samples a new column vector $\bar{h}^\ell_{b2a,\ell}$ consisting of $n'-\sum^{\ell-1}_{i=1} \hat{c}_i$ uniformly random group elements. 
                    
                    \item $\SIM_A$ further prepares another dummy set $\bar{h}^\ell_{a2b,\ell}$ which is initially empty. $\SIM_A$ sequentially enumerates each entry in the $i-th$ column of $\bar{H}^\ell_{B2A}$: if the $i$-th entry was chosen to be equal to some  $g_{i'j', A}$, then adds $\bar{h}^\ell_{b2a,\ell}[i]$ to $\bar{h}^\ell_{a2b,\ell}$. After this step, $\bar{h}^\ell_{a2b,\ell}$ should consist of $\hat{c}_\ell$ elements.
                    
                    \item $\SIM_A$ inserts independent and uniformly random group elements to $\bar{h}^\ell_{a2b,\ell}$ until it contains $m'-\sum^{\ell-1}_{i=1} \hat{c}_i$ group elements. Now for each element in $\bar{h}^\ell_{a2b,\ell}$, $\SIM_A$ raises it to the power of $\alpha_1 \cdot \alpha^{-1}_{\ell}$. $\SIM_A$ applies a random permutation to the resulting $\bar{h}^\ell_{a2b,\ell}$ and uses it as party $B$'s message $(h^\ell_{a2b,\ell})^{\alpha_1\beta_\ell}_{\pi_{B_\ell}}$ in Step 3.(3) of the protocol. 
                    \item $\SIM_A$ follows the protocol description honestly to perform Step 3.(4). 

                    \item $\SIM_A$ samples a uniformly random permutation $\pi_{A_\ell}$ to $(\bar{h}^\ell_{b2a,\ell})$ and uses the result as party $B$'s message $(h^\ell_{b2a,\ell})^{\alpha_\ell\beta_\ell}_{\pi_{A_\ell}}$ in Step 3.(5).    
                    
                    % \item $\SIM_A$ raises all the elements in $(\bar{h}^\ell_{b2a,\ell})$ to the power of $\alpha_\ell$, then samples a uniformly random permutation $\pi_{A_\ell}$ to it and uses the result as party $B$'s message $(h^\ell_{b2a,\ell})^{\alpha_\ell\beta_\ell}_{\pi_{A_\ell}}$ in Step 3.(5).                  
                    % \item Let $\bar{H}^\ell_{B2A}$, which has $n'-\sum^{\ell-1}_{i=1} \hat{c}_i$ rows, denote the matrix that simulates $H^\ell_{B2A}$ in the real protocol. To simulate Step 3.(3), $\SIM_A$ generates $(\bar{h}^\ell_{a2b,\ell})^{\alpha_1\bar{\beta}_\ell}_{\bar{\pi}_{B_\ell}}$ , where $\bar{\pi}_{B_\ell}$ is a random permutation. Note that all values required here ($\bar{h}^\ell_{a2b,\ell}, \alpha_1, \bar{\beta}_\ell$) are available to $\SIM_A$.
                    
                    % \item $\SIM_A$ follows the protocol description to perform Step 3.(4), except that the input $(h^\ell_{a2b,\ell})^{\alpha_1\bar{\beta}_\ell}_{\pi_{B_\ell}}$ is simulated by $\SIM_A$ instead of the actual input of party B.
                    % \item Similarly, to simulate Step 3.(5), $\SIM_A$ computes $(h^\ell_{b2a,\ell})^{\alpha_\ell\bar{\beta}_\ell}_{\pi_{A_\ell}}$. Note that all values required here ($h^\ell_{b2a,\ell}, \alpha_\ell, \bar{\beta}_\ell$) are available to $\SIM_A$.
                    
                    % \item $\SIM_A$ follows the protocol description honestly to perform Step 3.(4). 
                    
                    % \item $\SIM_A$ samples a uniformly random permutation $\pi_{A_\ell}$ and uses $(\bar{h}^\ell_{b2a,\ell})_{\pi_{A_\ell}}$ as party $B$'s message $(h^\ell_{b2a,\ell})^{\alpha_\ell\bar{\beta}_\ell}_{\pi_{A_\ell}}$ in Step 3.(5). 

                    \item  $\SIM_A$ follows the protocol description honestly to perform Step 3.(6) and Step 3.(7). 
                \end{enumerate}
            \end{itemize}


    \end{itemize}

    \end{minipage}    
}
    \caption{Description of $\SIM_A$ for Theorem~\ref{thm:dppsi}}
    \label{fig:sim_A_new}
\end{figure*}


We start with the definitions of the hybrid arguments:

\begin{itemize}
    \item $\hybrid_0$: The view of party $A$ in a real execution of the protocol.
    \item $\hybrid_{1,1,0}$: Identical to $\hybrid_0$. 
    \item $\hybrid_{1,1,i}$: For $i \in \{1,\ldots, m'-\hat{c}_1\}$, $\hybrid_{1,1,i}$ is the same as $\hybrid_{1,1,i-1}$, except with $(h_{\mathbf{a}_1}[i^\ast])^{\alpha_1\beta_1} = \hash(\mathbf{a}_1[i^\ast])^{\alpha_1\beta_1}$ replaced by $(g_{i^\ast})^{\alpha_1}$, where $h_{\mathbf{a}_1}[i^\ast]=\hash(\mathbf{a}_1[i^\ast])$ is the lexicographically smallest as-yet-unreplaced element which is not in the intersection set and $g_{i^\ast}$ is a random element.
    \item $\hybrid_{1,2,0}$: Identical to $\hybrid_{1,1,n'-\hat{c}_1}$.   
    \item $\hybrid_{1,2,i}$: For $i \in \{1,\ldots, m'-\hat{c}_1\}$, $\hybrid_{1,2,i}$ is the same as $\hybrid_{1,2, i-1}$, except with one element in the first column $H^1_{B2A}[1,i^\ast]$ replaced by $h_{i^\ast}$, where $H^1_{B2A}[1,i^\ast]$ is the lexicographically smallest as-yet-unreplaced element which is not in the intersection set and $h_{i^\ast}$ is a random element.
    \item $\hybrid_{1,3,0}$: Identical to $\hybrid_{2, m'-\hat{c}_1}$.
    \item $\hybrid_{1,3,i}$: For $i \in \{1,\ldots, \hat{c}_1\}$, $\hybrid_{1,3,i}$ is the same as $\hybrid_{1,3,i-1}$, except:
        \begin{itemize}
            \item $(h_{\mathbf{a}_1}[i^\ast])^{\alpha_1\beta_1}$ replaced by $g_{k^\ast}^{\alpha_1}$.
            \item $H^1_{B2A}[1,i^\ast]$ replaced by $g_{k^\ast}$.
        \end{itemize}
    where $i^\ast$ is the lexicographically smallest as-yet-unreplaced element which is in the intersection set. $g_{k^\ast}$ is a random element of $G$.

    \item $\hybrid_{1,4,0}$:Identical to $\hybrid_{1, 3,\hat{c}_1}$.   
    \item $\hybrid_{1,4,i}$:For $i \in \{1,\ldots, (L - 1)n'\}$, $\hybrid_{1,4,i}$ is identical to $\hybrid_{1,4,i-1}$, except with $H_{B2A}[i^\ast]$ replaced by $h_{i^\ast}$, where $H_{B2A}[i^\ast]$ is the index-wise smallest as-yet-unreplaced element from the second column of $H_{B2A}$ to the last column of $H_{B2A}$. $h_{i^\ast}$ is a random element.
\end{itemize}

We also define a sequence of transitional hybrids $(\hybrid_{\ell,1,0}$, $\ldots$, $ \hybrid_{\ell,1,m'-\sum^{\ell}_{k=1} \hat{c}_{k}})$ ,$(\hybrid_{\ell,2,0}$, $ \ldots$, $\hybrid_{\ell,2,n'-\sum^{\ell}_{k=1} \hat{c}_{k}})$, and $ (\hybrid_{\ell,3,0}$, $\ldots$, $\hybrid_{\ell,3,\hat{c}_{\ell}})$, for $\ell \in \{2, \ldots, L\}$. These arguments are used to represent the changes for each column of the input data.

\begin{itemize}
    \item $\hybrid_{\ell,1,0}$: $\hybrid_{\ell,1,0}$ is identical to $\hybrid_{\ell - 1,3,\hat{c}_{\ell - 1}}$. ($\hybrid_{2,1,0}$ is identical to $\hybrid_{1,4,(L - 1)n'}$.)
    
    \item $\hybrid_{\ell,1,i}$: For $i \in \{1,\ldots, m'-\sum^{\ell}_{k=1} \hat{c}_{k}\}$,  $\hybrid_{\ell,1,i}$ is the same as $\hybrid_{\ell,1,i-1}$, except with $(h^\ell_{a2b,\ell}[i^\ast])^{\alpha_1\beta_\ell}_{\pi_{B_\ell}}$ replaced by a $g_{i^\ast}^{\alpha_1\alpha_\ell^{-1}}$, where $h_{a2b,\ell}[i^\ast]$ is the lexicographically smallest as-yet-unreplaced element which is not in the intersection and $g_{i^\ast}$ is a random element.

    \item $\hybrid_{\ell,2,0}$: $\hybrid_{\ell,2,0}$ is identical to $\hybrid_{\ell,1,m'-\sum^{\ell}_{k=1} \hat{c}_{k}}$; 
    
    \item $\hybrid_{\ell,2,i}$: For $i \in \{1,\ldots, n'-\sum^{\ell}_{k=1} \hat{c}_{k}\}$,  $\hybrid_{\ell,2,i}$ is the same as $\hybrid_{\ell,2,i-1}$, except with $(h^\ell_{b2a,\ell}[i^\ast])^{\alpha_\ell\beta_\ell}_{\pi_{A_\ell}}$ replaced by  $h_{i^\ast}$, where $h^\ell_{b2a,\ell}[i^\ast]$ is the lexicographically smallest as-yet-unreplaced element which is not in the intersection and $h_{i^\ast}$ is a random element.

    \item $\hybrid_{\ell,3,0}$: $\hybrid_{\ell,3,0}$ is identical to $\hybrid_{\ell,2,n'-\sum^{\ell}_{k=1} \hat{c}_{k}}$; 

    \item $\hybrid_{\ell,3,i}$: For $i \in \{1,\ldots, \hat{c}_{\ell}\}$,  $\hybrid_{\ell,3,i}$ is the same as $\hybrid_{\ell,3,i-1}$, except :
        \begin{itemize}
            \item $(h^\ell_{a2b,\ell}[i^\ast])^{\alpha_1\beta_\ell}_{\pi_{B_\ell}}$ replaced by $g_{k^\ast}^{\alpha_1\alpha_\ell^{-1}}$.
            \item $(h^\ell_{b2a,\ell}[i^\ast])^{\alpha_\ell\beta_\ell}_{\pi_{A_\ell}}$ replaced by $g_{k^\ast}$.
        \end{itemize}
    where $i^\ast$ is the lexicographically smallest as-yet-unreplaced element which is in the intersection set. $g_{k^\ast}$ is a random element of $G$.
  \end{itemize}

\begin{itemize}
     \item $\hybrid_{final}$: The view of party $A$ otuput by $\SIM_A$.
 \end{itemize}

% In~\Cref{fig:sim_A} we describe the simulator $\SIM_A$. We claim that the distribution generated by $\SIM_A$ in the ideal world is indistinguishable from the output distribution of party $A$ in the real world. Our proof uses the standard hybrid argument, where neighboring pair of hybrid distributions is (computationally) indistinguishable. 

% \begin{itemize}
%     \item[$\hybrid_0$]: The view of party $A$ in a real execution of the protocol: $H^1_{B2A}$, $(h_{\mathbf{a}_1})^{\alpha_1\beta_1}_{\pi_{B_1}}$, and $(h^\ell_{a2b,\ell})^{\alpha_1\beta_\ell}_{\pi_{B_\ell}}$, $(h^\ell_{b2a,\ell})^{\alpha_\ell\beta_\ell}_{\pi_{A_\ell}}$ for $\ell \in {2, 3, \ldots, L}$.
%     \item[$\hybrid_{0,0}$]: Identical to $\hybrid_0$. 
%     \item[$\hybrid_{0,i}$]: For $i \in \{1,\ldots, n'\}$, $\hybrid_{1,i}$ is the same as $\hybrid_{1, i-1}$, except with $H_{B2A[i]}$ replaced by $\bar{H}_{B2A[i]}$.
%     \item[$\hybrid_{1,0}$]: Identical to $\hybrid_{0, n'}$.     
%     \item[$\hybrid_{1,i}$]: For $i \in \{1,\ldots, m'-\hat{c}_1\}$, $\hybrid_{1,i}$ is the same as $\hybrid_{1, i-1}$, except with $(h_{\mathbf{a}_1}[i^\ast])_{\pi_B}^{\alpha_1\beta_1}$ replaced by $(h_{\mathbf{a}_1}[i^\ast])_{\bar{\pi}_B}^{\alpha_1\bar{\beta}_1}$, where $(h_{\mathbf{a}_1}[i^\ast])_{\pi_B}^{\alpha_1\beta_1}$ is the lexicographically smallest as-yet-unreplaced element that is not in the intersection.
    
% \end{itemize}
% \noindent Similarly, we also define a sequence of transitional hybrids $((\hybrid_{a2b,2,0}, \ldots, \hybrid_{a2b, 2, m' - \sum_{i = 1}^{2} c_i}, \ldots, (\hybrid_{a2b, L,0}, \ldots, \hybrid_{a2b, L, m' - \sum_{i = 1}^{L} c_i})))$, for $\ell \in \{2, \ldots, L\}$:
% \begin{itemize}
%     \item[$\hybrid_{a2b,\ell,0}$:] $\hybrid_{a2b,\ell,0}$ is identical to $\hybrid_{\ell - 1,m' - \sum_{i = 1}^{\ell - 1} c_i}$ ($\hybrid_{a2b,2,0}$ is identical to $\hybrid_{1,m'-\hat{c}_1}$); 
%     % for $\ell \in [2,L]$, $\hybrid_{\ell,0}$ is identical to $\hybrid_{\ell-1, n'-\hat{c}_{\ell-1}}$.   
%     \item[$\hybrid_{a2b,\ell,i}$:] For $i \in \{1,\ldots, m'-\sum^{\ell-1}_{k=1} \hat{c}_{k}\}$,  $\hybrid_{\ell,i}$ is the same as $\hybrid_{\ell,i-1}$, except with $(h_{a2b,\ell}[i^\ast])_\pi^{\alpha_1\beta_\ell}$ replaced by $(\bar{h}_{a2b,\ell}[i^\ast])_\pi^{\alpha_1\bar{\beta}_\ell}$ where $(h_{a2b,\ell}[i^\ast])_\pi^{\alpha_1\beta_\ell}$ is the lexicographically smallest as-yet-unreplaced element that is not in the intersection set. % and $g_{i^\ast\ell, A}$ is a random element.
%   \end{itemize}

% \begin{itemize}
%     \item[$\hybrid_{b2a, \ell, 0}$:] Identical to $\hybrid_{b2a, \ell - 1,n'- \sum_{i = 1}^{\ell - 1} c_i}$. (Except that $\hybrid_{b2a, 2, 0} = \hybrid_{a2b,L,m' - \sum_{i = 1}^{L} c_i}$)
%     \item[$\hybrid_{b2a, \ell, i}$:] $i \in \{1,\ldots, n'-\sum^{\ell-1}_{k=1} \hat{c}_{k}\}$, $\hybrid_{b2a,\ell,i}$ is the same as $\hybrid_{b2a,\ell,i-1}$, except with $(h_{b2a,\ell}[i^\ast])_\pi^{\alpha_\ell\beta_\ell}$ being replaced by $(\bar{h}_{b2a,\ell}[i^\ast])_\pi^{\alpha_\ell\bar{\beta}_\ell}$, where $(h_{b2a,\ell}[i^\ast])_\pi^{\alpha_\ell\beta_\ell}$ is the lexicographically smallest as-yet-unreplaced element that is not in the intersection.
% \end{itemize}


% \begin{itemize}
%      \item[$\hybrid_{final}$:] The view of party $A$ otuput by $\SIM_A$.
%  \end{itemize}

\begin{algorithm}[!t] \footnotesize

\SetKwInOut{KIN}{Input}
\SetKwInOut{KOUT}{Output}
\caption{Simulator of $\hybrid_{1,1,i}$}
\label{alg:sim_ddh}
\KIN{$i$, $\alpha_1$, $g$, $g^a$, $g^b$, $g^c$, $\mathbf{a}_1 = (\mathbf{a}_1[1], \ldots, \mathbf{a}_1[m'])^T$, $\mathbf{b}_1 = (\mathbf{b}_1[1], \ldots, \mathbf{b}_1[n'])^T$}
\KOUT{The view of $SIM_A$ in $\hybrid_{1,1,i}$.}
% , $SIM_{\hybrid_{1,i}}(i^\ast, \alpha_1, g, g^a, g^b, g^c, \mathbf{a}_1, \mathbf{b}_1)$ with $\mathbf{a}_1[i^\ast]$ being the new element replaced with a random one in $\hybrid_{1,1,i}$}
Notation: $\mathbf{a}_1[i^\ast]$ is the new element replaced with a random one in $\hybrid_{1,1,i}$.

\For{$i \leftarrow 1$ to $m'$} {
    \If{ $\mathbf{a}_1[i] \neq \mathbf{a}_1[i^\ast]$}{
      Randomly sample $r_i \leftarrow \{1, \ldots, |\GG| \}$
      Program $H(\mathbf{a}_1[i])= g^{r_i}$
    }
    \ElseIf {$\mathbf{a}_1[i] = \mathbf{a}_1[i^\ast]$} {
      Program $H(\mathbf{a}_1[i])= g^{a}$
    }
}

\For{$j \leftarrow 1$ to $n'$} {
    \If{ $\mathbf{b}_1[j] \notin \mathbf{a}_1$}{
      Randomly sample $s_j \leftarrow \{1, \ldots, |\GG| \}$
      Program $H(\mathbf{b}_1[j])= g^{s_j}$
    }
}

Use $H$ as the random oracle in the protocol execution.
Initialize a vector $T = \{ t_1, \ldots, t_{m'} \}$.

\For{$i \leftarrow 1$ to $m'$} {
    \If{$\mathbf{a}_1[i] = \mathbf{a}_1[i^\ast]$} {
        $t_i = g^c$
    }
    \ElseIf {$\mathbf{a}_1[i] \notin \mathbf{b}_1, \mathbf{a}_1[i] < \mathbf{a}_1[i^\ast]$} {
    $t_i \leftarrow$ random element of $\GG$
    }
    \Else {
    $t_i = (g^b)^{s_i}$
    }
}

Shuffle and send $\{ t_i^{\alpha_1}\}_{i \in [m']}$ as Party B's message in Step 3.1.(3) of $SIM_A$.

Shuffle and send $\{(g^b)^{s_j}\}_{j \in [n']}$ as Party B's message in Step 3.1.(1) of $SIM_A$.

Honestly generate Party A's messages using party B's dummy messages from Step 3.1.(1).

Output party A's view in the simulated execution above.

\end{algorithm}

We argue that each consecutive pair of hybrids in the above sequence is indistinguishable by any PPT algorithm. 
The interesting arguments are $(\hybrid_{\ell,1,i},\hybrid_{\ell,1,i-1})$, $(\hybrid_{\ell,2,i},\hybrid_{\ell,2,i-1})$, $(\hybrid_{\ell,3,i},\hybrid_{\ell,3,i-1})$. 
They all follow a similar line of argument that relies on the hardness of DDH and the random oracle property of the hash function, we only go through one of the arguments as an example. 
In particular, we argue that for any PPT adversary $\mathcal{A}$ who can distinguish $(\hybrid_{1,1,i},\hybrid_{1,1,i-1})$, we can devise an adversary $\mathcal{B}$ to solve the DDH problem. 
$\mathcal{B}$ is given $(g, g^a, g^b, g^{c})$ and needs to decide whether $c$ is random or $c=ab$. 

We prove this argument by constructing an algorithm that takes a DDH tuple as the inputs, and outputs a simulation view of $\hybrid_{1,1,i}$. The algorithm is shown in Algorithm~\ref{alg:sim_ddh}.
First, we show that the output distribution produced by Algorithm~\ref{alg:sim_ddh} is identical to $\hybrid_{1,1,i}$. To begin with, we observe that the re-programed random oracle $H$ still has uniformly random output as all the re-programed values are random powers of a generator. Then, if we think of the value $b$ as the private key $\beta_1$ of party B, it can be seen that the un-replaced messages simulated for Step 3.1.(3) are of the format $H(\mathbf{b}_1[i])^{\alpha_1\beta_1}$, and the replaced messages are of the format $(g^{r})^{\alpha_1}$ where $r$ is uniformly random. Besides, the messages simulated for Step 3.1.(1) also follows the format of $H(\mathbf{b}_1)^{\beta_1}$. 

Now we replace the DDH tuple with $(g, g^a, g^b, g^{ab})$ and feed it to Algorithm~\ref{alg:sim_ddh} as the input. The only difference is that $t_{i^\ast} = g^c$ is replaced with $t_{i^\ast} = g^{ab} = H(\mathbf{a}_1[i^\ast])^b$. If we interpret $b$ as $\beta_1$, we can see that $t_{i^\ast}^{\alpha_1} = H(\mathbf{a}_1[i^\ast])^{\alpha_1\beta_1}$, which turns $t_{i^\ast}$ from replaced data to un-replaced data. This change is exactly the difference between $\hybrid_{1,1,i - 1}$ and $\hybrid_{1,1,i}$.

As a result, we can see that if there is an adversary that can distinguish between $\hybrid_{1,1,i - 1}$ and $\hybrid_{1,1,i}$, then it can also distinguish between $(g, g^a, g^b, g^c)$ and $(g, g^a, g^b, g^{ab})$ by observing the output distribution of Algorithm~\ref{alg:sim_ddh}. Therefore, as we assume the hardness of DDH, we conclude that $\hybrid_{1,1,i - 1}$ and $\hybrid_{1,1,i}$ have to be indistinguishable.

The proof of other hybrid argument pairs are similar and we omit the detailed proof here. For example, to build a DDH simulator for hybrid pairs $(\hybrid_{\ell,1,i},\hybrid_{\ell,1,i-1})$ for $\ell \neq 1$, you can simply replace $\{ t_i^{\alpha_1}\}_{i \in [m']}$ with $\{ t_i^{\alpha_1\alpha_\ell^{-1}}\}_{i \in [m' - \sum_{i = 1}^{\ell - 1} \hat{c}_i]}$ in line $18$ of Algorithm~\ref{alg:sim_ddh}.
\end{proof}

% \begin{sidewaysfigure*}[htbp!]
%     \begin{subfigure}
%     \centering
% \includegraphics[width=1\textwidth
% ]{images/AnonPSI-A.png}
%     \caption{DPCA-PSI}
%     \label{fig:DPCA-PSI-B}
%     \end{subfigure}
%     \begin{subfigure}
%     \centering
% \includegraphics[width=1\textwidth
% ]{images/AnonPSI-B.png}
%     \caption{DPCA-PSI}
%     \label{fig:DPCA-PSI-A}
%     \end{subfigure}
% \end{sidewaysfigure*}

\subsection{Experiments Setup}
~\label{app:implementation}

We use the Intel Paillier Cryptosystem Library (IPCL) library for fast homomorphic encryption operations. Besides, Openssl secp256r1 is chosen to support ECC operations. 
Besides, we use multi-threading %is fully leveraged 
to accelerate the elliptic curve operations. 
We compare our results with state-of-the-art PSI protocols~\cite{multi_key_meta} to illustrate better performance even with differential privacy protection. 
%This is achieved through better protocol design and a series of engineering optimizations and we will make the code open-source in the full version of this paper. 

The experiments are conducted on two desktop workstations equipped with $32$-core Intel(R) Xeon(R) Platinum 8336C CPU @ 2.30GHz and $128$GB RAM that enables AVX512IFMA instruction set. AVX512IFMA instruction set is used to support fast homomorphic encryption operations with the IPCL library, which improves the performance for the execution of  DPCA-PSI with payloads for subsequent MPC computation. Two servers are connected through LAN, and we make use of Linux's ``\texttt{tc}'' command to simulate the network settings with different latency and bandwidth. For each input set size, we simulate two settings: balanced settings where two parties have equal-size input set, and unbalanced settings where the ratio of the size of two parties' input sets is $10:1$\footnote{In unbalanced setting, we refer to the larger input set as the input size for all the following benchmark tables}.

\subsection{Comparison with Circuit-PSI}
\label{app:circuit-psi}
Adapting circuit-PSI protocols to support multi-ID matching is a significant challenge, especially with waterfall matching logic. Therefore, we only compare the performance with~\cite{popets/ChandranGS22} in the single-ID setting. 
We obtain their C++ implementation from GitHub and test their performance with the same hardware settings. Since our focus is on evaluating the performance of the PSI component, payloads are not included in this experiment. The benchmark results are presented in Table~\ref{tbl:benchmark_circuit_psi}. We observe that the main advantage of DPCA-PSI is the communication cost, which is around $10\times$ cheaper than Circuit-PSI. Consequently, DPCA-PSI performs much better than PSM2~\cite{popets/ChandranGS22}, especially in slower network settings. 
% Furthermore, when considering payloads, DPCA-PSI will demonstrate a more obvious advantage. This is because the input size of the downstream MPC in DPCA-PSI is determined by the intersection set size, which can be significantly smaller than that of circuit-PSI (the size of both parties' input sets).

\begin{table*}[!htbp]  \footnotesize
	\centering\setlength{\extrarowheight}{2pt}
	\caption{Performance comparison between DPCA-PSI and Circuit PSI~\cite{popets/ChandranGS22}. Each party has one column as the ID and no payloads. (PSM2 is the protocol presented in \cite{popets/ChandranGS22})}  
	\label{tbl:benchmark_circuit_psi}

	\begin{tabular} {c|r|r|r|r|r|r|r|r} %{|p{1.2cm}|p{1cm}|p{1cm}|p{1cm}|p{1cm}|p{1cm}|p{1cm}|p{1cm}|p{1cm}|}
		\toprule
		\multirow{3}*{Input size} & \multicolumn{6}{c|}{Time (sec)} &  \multicolumn{2}{c}{Comm. (MB)} \\ 
		\cline{2-7}
          & \multicolumn{2}{c|}{$10$Gb \& $0.2$ms} & \multicolumn{2}{c|}{$100$Mb \& $50$ms}& \multicolumn{2}{c|}{$10$Mb \& $50$ms} & \multicolumn{2}{c}{}\\
		\cline{2-9}
		 & PSM2 & DPCA-PSI & PSM2 & DPCA-PSI &PSM2 & DPCA-PSI &PSM2 & DPCA-PSI \\
         \hline
         $10^3 $ & $0.85$ & $0.71$ & $5.82$ & $2.66$ & $7.15$ & $4.27$ & $3.57$ & $0.11$ \\
         \hline
         $10^4 $ & $1.02$ & $1.07$ & $7.81$ & $3.47$ & $12.46$ & $4.72$ & $12.04$ & $0.89$ \\
         \hline
         $10^5 $ & $2.70$ & $2.33$ & $17.04$ & $6.10$ & $75.03$ & $12.42$ & $102.37$ & $8.62$ \\
         \hline
         $10^6 $ & $22.71 $ & $16.09$ & $89.78$ & $27.76$ & $672.75$ & $95.95$ & $1075.56$ & $85.57$ \\
         \hline
         $10^7 $ & $230.06$ & $163.28$ & $806.39$ & $241.95$ & $6305.37$ & $934.67$ & $10756.52$ & $858.36$ \\
         \bottomrule
	\end{tabular}
\end{table*}
